# Supplementary material for: When NAS Meets Trees: An Efficient Algorithm for Neural Architecture Search
Source: arXiv:2204.04918 source file (2022-04-11)
Supplement: Supplementary file 1 [file supplement.tex]

%  The same as previous methods, DAS-BT also have variance in search accuracy due to the random initialization. There are some architectures can have very close results, and are hard to be distinguished by training few epochs. In real deployment of our methods, one can always random initialize networks for multiple times, and choose the best architecture that ranks top the most time. This leads to a result with much less variation. 

%%%%%%%%% TITLE

% \title{The Third Paradigm of Neural Architecture Search:\\ NAS Meets Binary Trees}

\title{When NAS Meets Trees: \\A New Paradigm for Neural Architecture Search\\-- Supplementary Material --}

% \title{When Neural Architecture Search Meets Binary Trees: \\Remarkable Improvements on Accuracy and Efficiency}

\author{First Author\\
Institution1\\
Institution1 address\\
{\tt\small firstauthor@i1.org}
% For a paper whose authors are all at the same institution,
% omit the following lines up until the closing ``}''.
% Additional authors and addresses can be added with ``\and'',
% just like the second author.
% To save space, use either the email address or home page, not both
\and
Second Author\\
Institution2\\
First line of institution2 address\\
{\tt\small secondauthor@i2.org}
}

\maketitle

\setcounter{section}{0}

Here we provide additional information to supplement the main paper. We also attach a video to explain the paper.

\section{Exploration Size Analysis}
The number of architectures to score (exploration size $N$) is up bounded by $ \left( 2^{d_od_a}  \times  \left\lceil\frac{L}{d_a}\right\rceil  \times \left\lceil\frac{\log_2{(M-1)}+1}{d_o}\right\rceil  \right)$ in our proposed TNAS.  Here we list the exact number of $N$ of TNAS when using different expansion depths in \tblLabel \ref{table:darts_size}. 

\begin{table}[!htb]
    \centering
    \caption{Exploration size in the worst case in NAS-Bench-201 search space $L=6, M=5$. The maximum depth level of the binary operation tree is $\lceil\log_2(M-1)+1\rceil=3$. }.
    \label{table:darts_size}
    \resizebox{1.\columnwidth}{!}{
    \begin{tabular}{lc}
    \toprule
    Expansion depths & Exploration size\\ \midrule
	$d_a=1, d_o=1$ (progressive sequential greedy) & $2 \times 6 \times 3$=36\\
	$d_a=1, d_o=3$ (sequential greedy) & $5 \times 6 = 30$ \\
	$d_a=3, d_o=1$ & $2^3 \times \frac{6}{3} \times 3 = 48$ \\
	$d_a=6, d_o=1$ (progressive brute-force) &  $2^{6} \times 3 = 192$\\
	$d_a=6, d_o=3$ (brute-force) & $5^{6}= 15,625$ \\
    \bottomrule
    \end{tabular}
    }
\end{table}

\section{NAS-Bench-201 Details}
NAS-Bench-201 \cite{Dong2020NASBench201ET} builds a cell-based search space. The cell is a directed acyclic graph consisting of $4$ nodes and $L=6$ edges. Through our work, we denote each edge of the graph as an architecture layer. Each candidate network is stacked by $15$ cells. Each layer has an operation selected from $M=5$ operations. The search space contains $5^6 = 15,625$ candidate architectures in total. 
% All the candidates are reported with training, validation, and test accuracy on three datasets, CIFAR-10, CIFAR-100, and ImageNet-16-120.

\section{DARTS Search Space}

\subsection{Binary Operation Tree}
In DARTS search space, each architecture layer has $M=8$ operations for selection: $3\times3$ and $5\times5$ \textit{separable convolution}, $3\times3$ and $5\times5$ \textit{dilated separable convolution}, $3\times3$ \textit{maxpool}, $3\times3$ \textit{avgpool}, \textit{skip connection}, and \textit{none} (\textit{zero}).  The binary operation tree in DARTS operation space is illustrated in \figLabel \ref{fig:darts_operation_tree}. 

\begin{figure}[t]
\centering
\includegraphics[width=1.0\columnwidth]{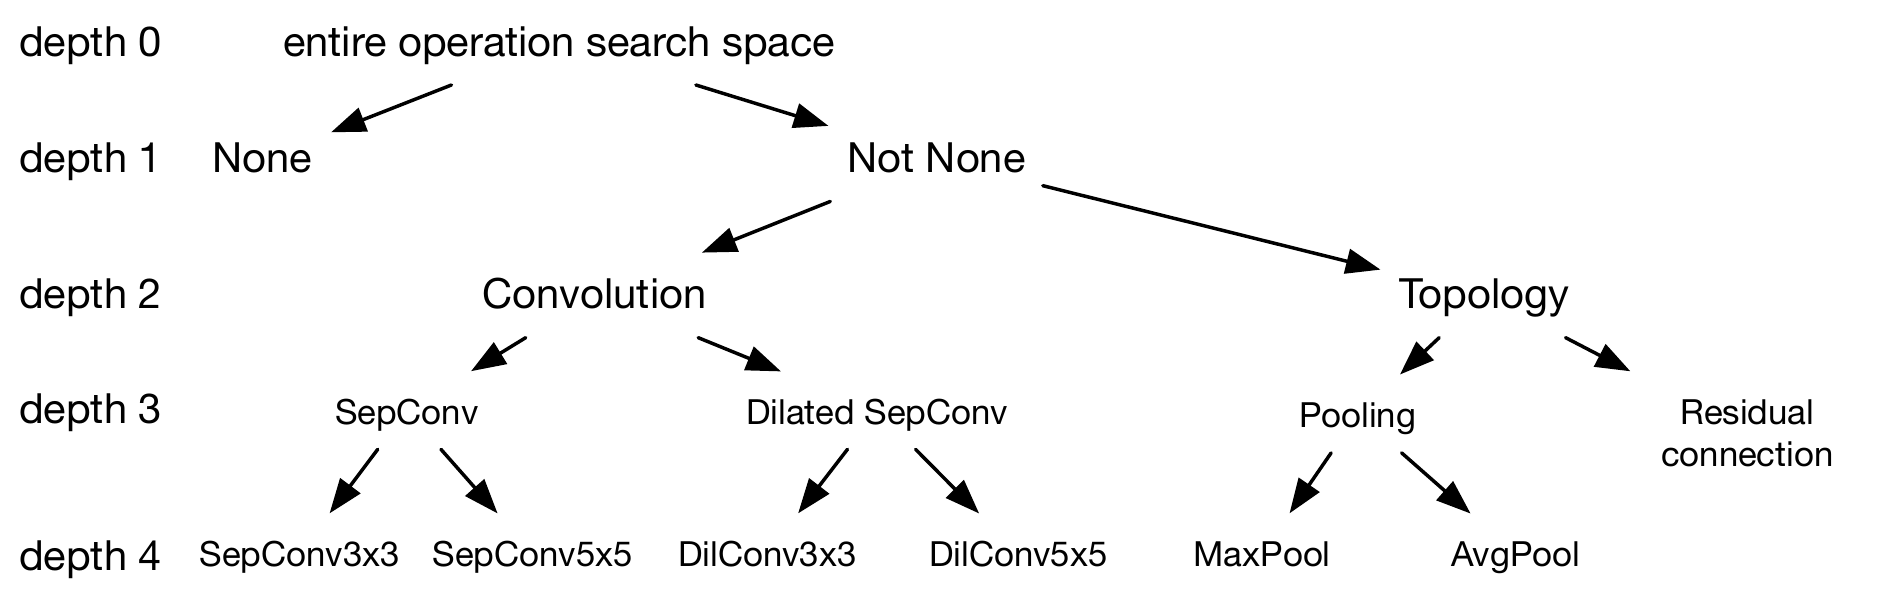}
\caption{\textbf{The binary operation tree $\mathcal{T}_O$} in DARTS operation space.
}
\label{fig:darts_operation_tree}
\end{figure}

\subsection{Architecture Trees}
Different from the NAS-Bench-201 \cite{Dong2020NASBench201ET}, in DARTS search space, one has to find the architectures for both normal cell and reduce cell. Each cell has $L=14$ layers.
We build an architecture tree for each cell. 
For each decision stage, our TNAS will search for the normal cell on the normal architecture tree at first, then search for the reduce cell on the reduce architecture tree, following our proposed TNAS algorithm.

\subsection{ImageNet Transfer}
We transfer the best cell architecture found in CIFAR-10 \cite{krizhevsky2009cifar10} to ImageNet \cite{imagenet_cvpr09} in the mobile setting. We adopt the same training and evaluation as DARTS \cite{liu2018darts}. We stack the found cells by $14$ times, and change the channel size to meet the 600M MAdds constraint. We train each network by $250$ epochs with label smoothing and an auxiliary classification head without other strong data augmentation. The results are shown in the main paper.

\subsection{Visualization of Architectures}
The best found cell architectures on CIFAR-10 \cite{krizhevsky2009cifar10} without the two incoming edges constraint are illustrated in \figLabel \ref{fig:architectures}. 

\begin{figure}[!htb]
\centering
\begin{subfigure}{\columnwidth}
\includegraphics[width=1.0\columnwidth]{figures/architectures/tnasl1_1_normal.pdf}
\caption{The best found Normal cell.
}
\end{subfigure}
\begin{subfigure}{\columnwidth}
\includegraphics[width=1.0\columnwidth]{figures/architectures/tnasl1_1_reduction.pdf}
\caption{The best found Reduce cell.
}
\end{subfigure}
\caption{\textbf{The best found architectures of TNAS in DARTS search space} \cite{liu2018darts}.}
\label{fig:architectures}
\end{figure}

\section{RobustDARTS Search Space}
To show the strength of TNAS, we also experiment on the RobustDARTS search space S4 proposed in \cite{ZelaESMBH20}. This space consists of two candidate operations $3\times3$ \textit{sepconv} and \textit{noise}.  The \textit{noise} is intentionally added and actively harms the performance and should not be selected. We show the architecture found by TNAS in RobustDARTS S4 space in \figLabel \ref{fig:s4_architectures}. While DARTS \cite{liu2018darts} and PC-DARTS \cite{xu2019pc} cannot distinguish the harmful noise operation, our TNAS does not choose any $noise$ in both normal cell and reduce cell. \tblLabel \ref{table:s4} show the quantitative results of TNAS, which demonstrates that our TNAS outperforms the state-of-the-art by a large margin.

\begin{table}[!htb]
\centering
\caption{\textbf{State-of-the-art comparison on RobustDARTS search space S4}. 
}
\vspace{-1em}
\label{table:s4}
\resizebox{1.0\columnwidth}{!}{%
\begin{threeparttable}
    \scriptsize
    \begin{tabular}{cccccccccc}
    \toprule
    \multicolumn{3}{c}{\textbf{DARTS} \cite{liu2018darts}} &\multicolumn{2}{c}{\textbf{R-DARTS \cite{ZelaESMBH20}}}
    &\multicolumn{2}{c}{\textbf{SDARTS \cite{chen2020stabilizing}}} &\multirow{2}{*}{\textbf{PC-DARTS} \cite{xu2019pc}}
    &\multirow{2}{*}{\textbf{DARTS-} \cite{chu2021darts-}}
    &\multirow{2}{*}{\textbf{TNAS (ours)}}\\
    \cmidrule(r){1-3}  \cmidrule(r){4-5}  \cmidrule(r){6-7}
    - &ES & ADA & DP & L2 & RS & ADV\\ 
     \midrule
    7.20 & 3.71 & 4.84 & 3.58 & 3.56 & 2.93 & 2.87 & 3.02 & 2.86 & \textbf{2.43} \\
    \bottomrule
    \end{tabular}%
\end{threeparttable}
	}
\end{table}

\begin{figure}[!htb]
\centering
\begin{subfigure}{\columnwidth}
\includegraphics[width=1.0\columnwidth]{figures/architectures/s4_tnas_normal.pdf}
\caption{The Normal cell.
}
\end{subfigure}
\begin{subfigure}{\columnwidth}
\includegraphics[width=1.0\columnwidth]{figures/architectures/s4_tnas_reduction.pdf}
\caption{The Reduce cell.
}
\end{subfigure}
\caption{\textbf{The architecture found by TNAS in RobustDARTS S4 search space} \cite{ZelaESMBH20}.}
\label{fig:s4_architectures}
\end{figure}
